# Supplementary material for: Safe Multi-Agent Reinforcement Learning with Bilevel Optimization in Autonomous Driving
Source: arXiv:2405.18209 source file (2024-05-28)
Supplement: Supplementary file 1 [file appendix.tex]

% \section{Appendix}
